# Supplementary material for: Emergence of a Renormalized $1/N$ Expansion in Quenched Critical Many-Body Systems
Source: arXiv:2010.08364 ancillary file (2021-03-25)
Supplement: Supplementary file 1 [file Supplemental_Material-2010.08364.pdf]

# *Supplemental material for*
# Emergence of a renormalized $1/N$ expansion in quenched critical many-body systems

Benjamin Geiger, Juan Diego Urbina, and Klaus Richter
*Institut für Theoretische Physik, Universität Regensburg, D-93040 Regensburg, Germany*
(Dated: December 14, 2020)

## Appendix A: Mean-field analysis

As there is ambiguity in the quantization of a mean field (MF) 'classical' limit due to ordering, one has to take care also in the definition of the classical limit when finite size corrections are concerned. We take the perspective that the MF description emerges from the Wigner phase space representation of expectation values and thus symmetric ordering of the bosonic operators is required before replacing them by coherent state phase space coordinates. This produces $\mathcal{O}(1/N)$ corrections in the Hamiltonian that are irrelevant for the dynamics but are essential to obtain the correct particle number and ground state energy in the quantization of the model.

After symmetrically ordering all products of bosonic operators in the Hamiltonian and replacing

$$\hat{b}_j \to \sqrt{n_j} e^{-i\theta_j}, \quad \hat{b}_j^\dagger \to \sqrt{n_j} e^{i\theta_j} \tag{A1}$$

one obtains the MF Hamiltonian

$$\begin{aligned} H_{\mathrm{MF}} = &-2J\sqrt{n_1 n_2}\cos(\theta_1-\theta_2) \\ &+ \frac{U}{2}\left[n_1^2+n_2^2-2(n_1+n_2)+1\right]. \end{aligned} \tag{A2}$$

As the classical analogue to the particle number $\tilde{N} = n_1 + n_2$ is conserved one can eliminate its phase using the canonical transformation

$$n = \frac{n_1-n_2}{2}, \qquad \varphi = \theta_1 - \theta_2, \tag{A3}$$

$$\tilde{N} = n_1+n_2, \qquad \varphi_{\tilde{N}} = \frac{\theta_1+\theta_2}{2}. \tag{A4}$$

A closer analysis of the classical dynamics similar to the one performed in [1] shows that $\tilde{N}$ is the sum of the two action variables and thus should be quantized as $\tilde{N} = (m_1 + 1/2) + (m_2 + 1/2) \equiv N + 1$, where $m_1, m_2$ are the quantum numbers associated with the quantized actions. This explains the distinction between $\tilde{N}$ and $N$ in the main text, although it is not essential for the further analysis. With a final scale transformation defining

$$z = \frac{n}{\tilde{N}}, \quad h = \frac{H_{\mathrm{MF}} - H_{\mathrm{MF}}|_{n=\varphi=0}}{J\tilde{N}} \tag{A5}$$

one obtains the result in Eq. (4) of the main text.

## Appendix B: Coefficients of the $\hbar_{\mathrm{eff}}$ expansion

Indexing the expansions of the $n$ nonlinear potentials by subscripts $i = 1, \dots, n$ and expanding the operator $\hat{A}$ similarly as

$$\hat{A}(t) = \sum_{\mu_0,\nu_0} a_{\mu_0\nu_0} \hbar_{\mathrm{eff}}^{\frac{\mu_0+\nu_0}{2}} e^{(\nu_0-\mu_0)\lambda t} \hat{b}_-^{\mu_0} \hat{b}_+^{\nu_0} \tag{B1}$$

one finds

$$\hat{A}_H(t) = \sum_{n=0}^{\infty}\left(\prod_{i=0}^{n}\sum_{\mu_i,\nu_i}\right)\frac{c^{(n)}_{\boldsymbol{\mu\nu}}}{\lambda^n} f^{(n)}_{\boldsymbol{\mu\nu}}(\lambda t)\hbar_{\mathrm{eff}}^{\frac{\mu+\nu}{2}-n}\hat{B}^{(n)}_{\boldsymbol{\mu\nu}}, \tag{B2}$$

with $\mu = \sum_{i=0}^n \mu_i$, $\nu = \sum_{i=0}^n \nu_i$, $c^{(n)}_{\boldsymbol{\mu\nu}} = a_{\mu_0\nu_0}\prod_{i=1}^n v_{\mu_i\nu_i}$,

$$f^{(n)}_{\boldsymbol{\mu\nu}}(x) = \int_0^x dx_1 \int_0^{x_1} dx_2 \cdots \int_0^{x_{n-1}} dx_n \prod_{i=0}^{n} e^{(\nu_i-\mu_i)x_i} \tag{B3}$$

and the nested commutator

$$\hat{B}^{(n)}_{\boldsymbol{\mu\nu}} = (-i)^n[[\dots[[\hat{b}_{\mu_0\nu_0}, \hat{b}_{\mu_1\nu_1}], \hat{b}_{\mu_2\nu_2}], \dots], \hat{b}_{\mu_n\nu_n}] \tag{B4}$$

of the symmetrically ordered products

$$\hat{b}_{\mu\nu} = \{\hat{b}_-^{\mu}\hat{b}_+^{\nu}\}_{\mathrm{s}}. \tag{B5}$$

Using symmetric ordering is conventional and leads to simplifications later.

### 1. Proof of Eq. (15)

One now needs to identify the sets of coefficients $\{\mu_i, \nu_i \mid i = 0, \dots, n\}$ associated with the largest growth rate for a fixed exponent of $\hbar_{\mathrm{eff}}$.

*a. The time-integration:* By introducing the parameters

$$\eta_j = \sum_{i=0}^{j}(\nu_i - \mu_i), \tag{B6}$$

one can rewrite the time integrals as an $n$-fold convolution

$$f^{(n)}_{\boldsymbol{\mu\nu}} = g_{\eta_0} * g_{\eta_1} * \cdots * g_{\eta_n}, \quad g_\eta(x) = \begin{cases} e^{\eta x} & x \geq 0 \\ 0 & x < 0 \end{cases} \tag{B7}$$

that can be evaluated in closed form [2] leading to

$$f^{(n)}_{\boldsymbol{\mu\nu}}(x) = \sum_{\eta\in\mathcal{E}} g_\eta^{(m_\eta-1)}(x) e^{\eta x}, \tag{B8}$$

where $\mathcal{E}$ is the set of (different) values of the parameters $\eta_j$, now equipped with the multiplicities $m_\eta$, and

$$g_\eta^{(m_\eta-1)}(x) = \sum_{k=0}^{m_\eta-1} c_\eta^{(k)} \frac{x^{m_\eta-1-k}}{(m_\eta-1-k)!} \tag{B9}$$

is a polynomial in $x$ of order $m_\eta - 1$ with the constants $c_\eta^{(k)}$ generated by

$$\sum_{k=0}^{\infty} c_\eta^{(k)} z^k = \prod_{\eta' \in \mathcal{E}\setminus\{\eta\}} (z+\eta-\eta')^{-m_{\eta'}}. \tag{B10}$$

*b. The nested commutator:* The symmetrically ordered product has the advantage that it allows for the use of certain commutator relations. One finds for symmetrically ordered operators $\hat{A}, \hat{B}$ the formal rule

$$\left[\hat{A}, \hat{B}\right] = 2i \left\{ \hat{A} \sin\left(\frac{1}{2}\left(\overleftarrow{\partial}_{\hat{b}_-}\overrightarrow{\partial}_{\hat{b}_+} - \overleftarrow{\partial}_{\hat{b}_+}\overrightarrow{\partial}_{\hat{b}_-}\right)\right)\hat{B}\right\}_{\mathrm{s}}, \tag{B11}$$

which is the operator analogue of the Moyal bracket using $[\hat{b}_-, \hat{b}_+] = i$. Applying Eq. (B11) to (B4) and requiring a non-vanishing result directly leads to the bounds

$$\mu'_j = \sum_{i=0}^{j} \mu_i - j \geq 0, \qquad \nu'_j = \sum_{i=0}^{j} \nu_i - j \geq 0, \tag{B12}$$

i.e., the first $j$ commutators have to contain at least $j$ of the operators $\hat{b}_\pm$ each.

*c. Unique largest exponent:* We will now show that for a fixed exponent

$$k = \mu + \nu - 2n \tag{B13}$$

of $\sqrt{\hbar_{\mathrm{eff}}}$ in the expansion (B2) the growth rates $\eta$ in Eq. (B8) are bounded by $k$ and that this value can only be taken once, i.e.,

$$\eta \leq \eta_{\max} = k, \qquad m_{\eta_{\max}} \leq 1. \tag{B14}$$

By construction we have $v_{\mu\nu} = 0$ for $\mu + \nu \leq 2$. To directly implement this constraint it is convenient to rewrite the sums in Eq. (B2) as

$$\sum_{\substack{\mu_i,\nu_i \\ \mu_i+\nu_i>2}} F(\mu_i,\nu_i) = \sum_{M_i>2}\sum_{\mu_i=0}^{M_i} F(\mu_i, M_i-\mu_i) \tag{B15}$$

for $i \geq 1$, where $M_i = \nu_i + \mu_i$. Let us assume that all other expansion coefficients $v_{\mu\nu}$ and $a_{\mu\nu}$ are nonzero. Fixing $n$ and all the $M_i$, the exponents $\eta_j$, Eq. (B6), can only be varied by changing the $\mu_i$. A decrease in any of the $\mu_i$ then results in an increase of all the $\eta_j$ for $j \geq i$. In particular, one has

$$\eta_j = \sum_{i=0}^{j}(M_i - 2\mu_i) = \sum_{i=0}^{j} M_i - 2(\mu'_j + j). \tag{B16}$$

One can therefore maximize all the $\eta_j$ simultaneously by choosing $\mu'_j = 0$ according to Eq. (B12) leading to

$$\eta_j^{(\max)} \equiv \left[\sum_{i=0}^{j} M_i - 2j\right] \tag{B17}$$

$$= \eta_{j-1}^{(\max)} + \underbrace{(M_j - 2)}_{>0} > \eta_{j-1}^{(\max)} \tag{B18}$$

for $j \geq 1$. This shows that the largest possible exponent is given by

$$\eta_{\max} = \eta_n^{(\max)} = \mu + \nu - 2n = k \tag{B19}$$

and that $m_{\eta_{\max}} = 1$. As this is true for any (valid) choice of $n$ and the $M_i$ this proves the relation between Eq. (B13) and Eq. (B14). Moreover, it shows that the bound is taken in generic cases where $a_{\mu\nu}, v_{\mu\nu} \neq 0$.

*d. Calculation of the leading order:* For $\mu'_n = 0$ all but the first order of the sine function in Eq. (B11) vanish when applied to Eq. (B4), leading to

$$\hat{B}_{\boldsymbol{\mu\nu}}^{(n)} = \prod_{k=1}^{n} \begin{vmatrix} \mu'_{k-1} & \mu_k \\ \nu'_{k-1} & \nu_k \end{vmatrix} \hat{b}_+^k = \prod_{k=1}^{n} \begin{vmatrix} \mu'_{k-1} & \mu'_k+1 \\ \nu'_{k-1} & \nu'_k+1 \end{vmatrix} \hat{b}_+^k. \tag{B20}$$

One therefore obtains from Eq. (B2)

$$\hat{A}_H(t) = \sum_{k=0}^{\infty} C_k \left(\sqrt{\hbar_{\mathrm{eff}}} e^{\lambda t}\right)^k \left(\hat{b}_+^k + \mathcal{O}(te^{-\lambda t})\hat{b}_-^{l_1}\hat{b}_+^{l_2}\right) \tag{B21}$$

with $l_1 + l_2 \leq k$.

## 2. Calculation of $C_k$

The coefficient $C_k$ can contain a large but finite number of different terms. Let the smallest non-vanishing order of $v(\varphi, z)$ be given by $M > 2$, i.e., one can take $M_i \geq M$ for $i = 1, \ldots, n$ and let $m \geq 0$ be the smallest nonvanishing order of $A(\varphi, z)$ for $i = 0$. The terms contributing to the $C_k$ in Eq. (B21) will then have

$$k = \sum_{i=0}^{n} M_i - 2n \geq m + (M-2)n \Leftrightarrow n \leq \left\lfloor \frac{k-m}{M-2} \right\rfloor. \tag{B22}$$

For given values of $n$ and the $M_i$ there are several choices of the $\mu_i$ consistent with $\mu'_n = 0$. One finds

$$C_k = \sum_{n=0}^{\left\lfloor \frac{k-m}{M-2} \right\rfloor} \sum_{\boldsymbol{M} \in I_n^k} \sum_{\boldsymbol{\mu} \in J_n(\boldsymbol{M})} \frac{c_{\boldsymbol{\mu\nu}}^{(n)}}{\lambda^n} D_{\boldsymbol{\mu\nu}}^{(k)} \tag{B23}$$

with [cf. Eq. (B12)]

$$D_{\boldsymbol{\mu\nu}}^{(k)} = \prod_{j=1}^{n} \begin{vmatrix} \mu'_{j-1} & \mu'_j+1 \\ \nu'_{j-1} & \nu'_j+1 \end{vmatrix} (k - \nu'_{j-1} + \mu'_{j-1})^{-1}. \tag{B24}$$

The index set $I_n^k$ contains the tuples $(M_0,\ldots,M_n)$ summing up to $k+2n$ with $M_0 \geq m$ and $M_i \geq M > 2$ for $i=1,\ldots,n$. The set $J_n(\boldsymbol{M})$ contains the tuples $(\mu_0,\ldots,\mu_n)$ with $0 \leq \mu_i \leq M_i$ for $i=0,\ldots,n$ and with the further constraints

$$j \leq \sum_{i=0}^{j} \mu_i \leq \sum_{i=0}^{j} M_i - j, \tag{B25}$$

i.e., Eq. (B12), for $j < n$ and $\sum_{i=0}^{n} \mu_i = n$. The second inequality ensures

$$\nu_j' = \sum_{i=0}^{j} (M_i - \mu_i) - j \geq 0. \tag{B26}$$

Note that the index $n$ on $J_n$ can be omitted, as $n$ is encoded in the length of $\boldsymbol{M}$.

### 3. Matrix elements, expectation values and cumulants

The behavior of the matrix elements in Eq. (1) of the main text is only the leading order approximation in a series

$$\langle k|\hat{A}(t)|l\rangle = \sum_{m\geq 0} c_{kl}^{(m)} (\sqrt{\hbar_{\text{eff}}} e^{\lambda t})^{|k-l|+2m}, \tag{B27}$$

where, by virtue of Eq. (B21), one finds

$$c_{kl}^{(m)} = C_{|k-l|} \langle k|\hat{b}_+^{|k-l|+2m}|l\rangle. \tag{B28}$$

For completeness, the matrix elements in Eq. (B28) are reported here as (abbreviating $r=|k-l|+2m$)

$$\langle k|\hat{b}_+^r|l\rangle = \frac{r!}{m!\sqrt{k!l!}} \frac{e^{i(k-l)\phi}}{[2\sin(2\phi)]^{\frac{r}{2}}} \gamma_{kl}^{(m)},$$
$$\gamma_{kl}^{(m)} = \partial_z^{\min(k,l)} (1+z)^{\max(k,l)} \left(\frac{1}{2}+z\right)^m \Bigg|_{z=0} \tag{B29}$$

with the leading order coefficient for $m=0$ in Eq. (1) of the main text given by

$$c_{kl} \equiv c_{kl}^{(0)} = C_{|k-l|} \frac{\max(k,l)!}{\sqrt{k!l!}} \frac{e^{i(k-l)\phi}}{[2\sin(2\phi)]^{\frac{|k-l|}{2}}}. \tag{B30}$$

In the case of expectation values in thermal ensembles described by the density matrix

$$\hat{\rho}_0(\beta) = \frac{e^{-\beta\hat{h}_0}}{Z(\beta)}, \quad Z(\beta) = \mathrm{Tr}\left[e^{-\beta\hat{h}_0}\right], \tag{B31}$$

the description can be drastically simplified using Wick's theorem that applies due to the quadratic form of $\hat{h}_0$, Eq. (5) in the main text. In the current context it straightforwardly yields

$$\langle \hat{b}_+^{2m}\rangle = (2m-1)!\langle \hat{b}_+^2\rangle^m, \quad \langle \hat{b}_+^{2m-1}\rangle = 0 \tag{B32}$$

for $m \in \mathbb{N}$ and with

$$\langle \hat{b}_+^2\rangle = \frac{\coth\left(\frac{\beta\hbar_{\text{eff}}\omega}{2}\right)}{2\sin(2\phi)} \tag{B33}$$

being closely related to the imaginary-time Green's function evaluated at equal (imaginary) times. As the explicit dependence on $\hbar_{\text{eff}}$ is an artifact of the formal classical limit here, it is more convenient to write $\hbar_{\text{eff}}\omega = \Delta$ for the elementary excitation. Clearly, the above is not valid at arbitrary temperatures and, as will be shown in the next section, the harmonic approximation can be justified only if $\beta\Delta = \mathcal{O}(\hbar_{\text{eff}}^0)$.

The $n$-th cumulant $\kappa_n$ of an observable $\hat{O}$ is generated by

$$K_{\hat{O}}(z) = \log\langle e^{z\hat{O}}\rangle = \sum_{n=1}^{\infty} \frac{\kappa_n}{n!} z^n. \tag{B34}$$

Using $\hat{O} = \hat{A}(t)$ given in Eq. (15) of the main text one can use a general result [3] on the cumulants of functions of random variables that directly yields the scaling stated in Eq. (21) the main text. A more physical picture is obtained for a general expansion

$$\hat{O} = \sum_k c_k \hat{b}_+^k, \tag{B35}$$

interpreting $\hat{b}_+$ as a real scalar field. In a diagrammatic expansion of $Z = \langle \exp(z\hat{O})\rangle$, each $c_k$ defines a $k$-vertex, connected to other vertices via the 'propagator' $\langle \hat{b}_+^2\rangle$ associated with a particle line. As is the case in other diagrammatic expansions of partition functions, taking the logarithm eliminates all disconnected diagrams on a purely combinatorial level. The parameter $z$ in the cumulant generating function $K_{\hat{O}}(z)$ only introduces a method for counting vertices in the diagrammatic representation, such that the cumulant $\kappa_n$ consists of all connected diagrams with exactly $n$ vertices, and the smallest possible number of particle lines to connect all of them is given by $n-1$. Applying this result to the cumulant of $\hat{A}(t)$ in Eq. (15) in the main text, it is clear that each particle line $\langle \hat{b}_+^2\rangle$ also leads to a factor $\hbar_{\text{eff}} e^{2\lambda t}$, thus resulting in the scaling stated in the main text.

## Appendix C: Deviations from harmonica oscillator states

The actual noninteracting Hamiltonian used in the main text is not a harmonic oscillator and its eigenstates are *not* harmonic oscillator states. (Although the eigenstates of the noninteracting (quadratic) system used in the main text are harmonic, the excitations within a sector with fixed particle number are described by a spin with total spin quantum number $N/2$, as suggested also by the finite dimension of the projected Hilbert space.)

Let $|n\rangle$ denote the harmonic oscillator states, i.e., eigenstates of $\hat{h}_0$, Eq. (5) of the main text, and $|\psi_n\rangle$ denote the eigenstates of the full noninteracting Hamiltonian

$$\hat{h}_{\alpha=0} = \hat{h}_0 + \hat{v}_0. \tag{C1}$$

Note that for the special case of the two-site BH model used in the main text one even has $\hat{v}_0 = \hat{v}$, as the interaction only affects the quadratic terms. The two sets of eigenstates can be related via adiabatic switching [4]. For this one defines

$$\hat{U}_\epsilon = \hat{T} \exp\left( -\frac{i}{\hbar_{\text{eff}}} \int_{-\infty}^{0} dt\, e^{\epsilon t} \hat{v}_{0,I}(t) \right), \tag{C2}$$

where the operators in the interaction picture are now defined by the harmonic oscillator Hamiltonian,

$$\hat{v}_{0,I}(t) = e^{\frac{i}{\hbar_{\text{eff}}}\hat{h}_0 t} \hat{v}_0 e^{-\frac{i}{\hbar_{\text{eff}}}\hat{h}_0 t}. \tag{C3}$$

Then, assuming a one-to-one correspondence of the low-lying states, the Gell-Mann and Low theorem guarantees that

$$|\langle \psi_k|\hat{A}(t)|\psi_l\rangle| = \lim_{\epsilon\to 0} |\langle k|\hat{U}_\epsilon^\dagger \hat{A}(t)\hat{U}_\epsilon|l\rangle|. \tag{C4}$$

The absolute value has to be taken to cancel an infinite phase that appears in the limit (for $k \neq l$). For finite $\epsilon$ one can now expand $\hat{U}_\epsilon^\dagger \hat{A}(t)\hat{U}_\epsilon$ similar to Eq. (B2), with the only difference that instead of the operators $\hat{b}_\pm$ one now has to use $\hat{a}, \hat{a}^\dagger$, $\lambda$ is replaced by $\omega$, and the function $f_{\boldsymbol{\mu\nu}}(x)$ is replaced by

$$f_{\boldsymbol{\mu\nu}}(\epsilon) = \int_{-\infty}^{0} dx_1 \cdots \int_{-\infty}^{x_{n-1}} dx_n \prod_{j=1}^{n} e^{i(\nu_j - \mu_j - i\frac{\epsilon}{\omega})x_j}. \tag{C5}$$

The (Heisenberg) operator $\hat{A}(t)$ can thereby be taken as Eq. (B21) with $\hat{b}_+$ expressed by $\hat{a}$ and $\hat{a}^\dagger$ (the interaction picture and Heisenberg picture coincide at $t = 0$). With the same arguments as in the previous section one then finds that the expansion in powers of $\hbar_{\text{eff}}$ only contains terms of the form

$$\hbar_{\text{eff}}^{\frac{k'}{2}} e^{k\lambda t} \left\{ (\hat{a})^{l_1} (\hat{a}^\dagger)^{l_2} \right\}, \quad l_1 + l_2 \leq k' \tag{C6}$$

with coefficients that depend on the parameter $\epsilon$ and bounded functions in time, and $k$ being the order of $\sqrt{\hbar_{\text{eff}}}$ in Eq. (B21). For fixed order $n$ in $\hat{v}_0$ one has the relation

$$k' = \begin{cases} k + \sum_{i=1}^{n}(\mu_i + \nu_i) - 2n, & n \geq 1 \\ k, & n = 0. \end{cases} \tag{C7}$$

Using that $\hat{v}_0$ is at least cubic in the operators $\hat{a}, \hat{a}^\dagger$ one directly finds $k' > k$ for $n \geq 1$, but $k' = k$ for $n = 0$. Thus, one finds that the matrix element in Eq. (C4) also has

$$\langle k|\hat{U}_\epsilon^\dagger \hat{A}(t)\hat{U}_\epsilon|l\rangle \sim \sum_{m\geq 0} c_{kl}^{(m)} \left( \sqrt{\hbar_{\text{eff}}} e^{\lambda t} \right)^{|k-l|+2m} \times \left[ 1 + h_m(\epsilon, t)\mathcal{O}(e^{-2\lambda t}) \right] \tag{C8}$$

for $1 \ll \lambda t \ll \log \hbar_{\text{eff}}^{-1/2}$ with a $\hbar_{\text{eff}}$-independent function $h_m(\epsilon, t)$ that is bounded in time and the coefficients $c_{kl}^{(m)}$ given in Eq. (B28). As all of the above is valid for all $\epsilon$, it also holds for the limit in Eq. (C4) (that is assumed to exist for the low-lying states) and the undetermined phase only enters $h_m(\epsilon)$ in subdominant terms that can be neglected, thus yielding

$$\langle \psi_k|\hat{A}(t)|\psi_l\rangle \sim \langle k|\hat{A}(t)|l\rangle \tag{C9}$$

for $\lambda^{-1} \ll t \ll t_E$. As this holds for all states $|k\rangle$ with $k = \mathcal{O}(N^0)$ one can also replace thermal initial states with temperatures $k_B T/\Delta = \mathcal{O}(N^0)$ in terms of the level spacing $\Delta$. One can show this more formally by means of thermal field theory, treating the nonlinear parts of the pre-quench Hamiltonian as a perturbation and using $\hbar_{\text{eff}}\omega\beta = \hbar_{\text{eff}}\omega/k_B T = \mathcal{O}(\hbar_{\text{eff}}^0)$. Expanding an operator $\hat{A}$ in the bosonic operators $\hat{a}, \hat{a}^\dagger$ then yields

$$\langle \hat{A} \rangle = \langle \hat{A} \rangle_0 + \mathcal{O}(\hbar_{\text{eff}}^2). \tag{C10}$$

This can then be applied to the expansion of $\hat{A}(t)$ in terms of the time-independent operators $\hat{b}_+$, where the $\mathcal{O}(\hbar_{\text{eff}}^2)$ corrections become subdominant compared to the exponential terms.

## Appendix D: Extension to the $L$-site BH model

The results are easily generalized to the one-dimensional BH model with $L$ sites and periodic boundary conditions,

$$\hat{H} = -J \sum_{j=1}^{L} \left( \hat{b}_j^\dagger \hat{b}_{j+1} + \hat{b}_{j+1}^\dagger \hat{b}_j \right) + \frac{U}{2} \sum_{j=1}^{L} \hat{b}_j^\dagger \hat{b}_j^\dagger \hat{b}_j \hat{b}_j. \tag{D1}$$

Note that in the case of two sites one has to replace $J \to J/2$ due to double counting. The higher-dimensional cases (square and cubic lattice) can be obtained in the same manner but are not included here for brevity.

Ignoring any $\mathcal{O}(1/N)$ terms that can occur due to different orderings one finds the MF Hamiltonian

$$h = \frac{H_{\text{MF}}}{J\tilde{N}} = -\sum_{j=1}^{L} \left[ 2\sqrt{z_j z_{j+1}} \cos(\theta_j - \theta_{j+1}) + L\alpha z_j^2 \right], \tag{D2}$$

where the $z_i = n_i/\tilde{N}$ are the occupation fractions of the individual sites, $\tilde{N} = \sum_j n_j$, and $\alpha = -U\tilde{N}/(2JL)$. Varying this Hamiltonian with the constraint $\sum_j z_j = 1$ one finds a stationary point at

$$z_j = \frac{1}{L}, \quad \theta_j = \theta \tag{D3}$$

for $j = 1, \ldots, L$, where the global phase $\theta$ is arbitrary and reflects the $U(1)$ symmetry of the Hamiltonian. This holds irrespective of the value of $\alpha$, but the stability

properties of this point change. The quadratic expansion around this fixed point yields

$$\left.\frac{\partial^2 h}{\partial z_j \partial z_k}\right|_{\mathrm{FP}} = \frac{L}{2}\left(2\delta_{kj} - \delta_{kj+1} - \delta_{kj-1}\right) - 2L\alpha\delta_{kj}, \quad \text{(D4)}$$

$$\left.\frac{\partial^2 h}{\partial \theta_j \partial \theta_k}\right|_{\mathrm{FP}} = \frac{2}{L}\left(2\delta_{kj} - \delta_{kj+1} - \delta_{kj-1}\right), \quad \text{(D5)}$$

with the mixed derivatives vanishing. Decoupling the dynamics is straightforward using plane waves, resulting in the Hamiltonian

$$h = -(2+\alpha) + \sum_{k=0}^{L-1} h_k, \quad \text{(D6)}$$

$$h_k = 2\sin^2(\pi k/L)\left(\bar{\theta}_k^2 + \bar{z}_k^2\right) - 2\alpha \bar{z}_k^2, \quad \text{(D7)}$$

where

$$\bar{z}_k = \sqrt{\frac{L}{2}} \sum_{j=1}^{L} b_j^{(k)} (z_j - 1/L),$$

$$\bar{\theta}_k = \sqrt{\frac{2}{L}} \sum_{j=1}^{L} b_j^{(k)} (\theta_j - \theta), \quad \text{(D8)}$$

$$b_j^{(k)} = \begin{cases} \sqrt{2/L}\cos(2\pi jk/L) & 0 < k < L/2, \\ \sqrt{2/L}\sin(2\pi jk/L) & L/2 < k < L, \\ 1/\sqrt{L}(-1)^{2jk/L} & 2k = 0, L. \end{cases} \quad \text{(D9)}$$

Apart from $k = 0$ (corresponding to the conserved particle number) the $h_k$ are harmonic oscillators for $\alpha = 0$ and turn into inverted oscillators at

$$\alpha_k = \sin^2(\pi k/L) \quad \text{(D10)}$$

with the (in)stability exponents

$$\lambda_k = 4\sqrt{\alpha_k(\alpha - \alpha_k)}, \quad \text{(D11)}$$

for $\alpha > \alpha_k$ that come in pairs (as $\lambda_k = \lambda_{L-k}$), such that for $\alpha > 1$ one is left with $\lfloor L/2 \rfloor$ different stability exponents, e.g., for $L = 3$ one has $\alpha_1 = \alpha_2 = 3/4$ and $\lambda_1 = \lambda_2 = \sqrt{12\alpha - 9}$.

One can then proceed in the same way as in the two-site BH model by quantizing $[\hat{\bar{\theta}}_k, \hat{\bar{z}}_k] = i\hbar_{\mathrm{eff}}$ and expanding the nonlinear dynamics perturbatively, now leading to an exponential growth governed by integer linear combinations of the stability exponents with the sum of their coefficients being bound by the exponent of $\sqrt{\hbar_{\mathrm{eff}}}$ as before. However, for a consistent approximation that neglects terms that are $\mathcal{O}(e^{-\lambda_k t})$ for each $k$, only the largest stability exponent(s) may be used.

## Appendix E: Explicit leading order short-time results

In leading order in $\hbar_{\mathrm{eff}}$ one can easily calculate also the $\mathcal{O}(te^{\lambda t})$ corrections in Eq. (B21), as it does not depend on the nonlinear dynamics given by $\hat{v}$ that can only contribute to $\mathcal{O}(\hbar_{\mathrm{eff}}^{(M-1)/2})$ with $M > 2$ as before [see also Eq. (B22)]. In the BH models considered here one even has $M = 4$ such that the first two orders can be obtained from the zero order perturbation theory, i.e., they can be calculated using the linearized dynamics. For the two-site BH model one obtains to leading order the Heisenberg operators

$$\begin{pmatrix} \hat{\varphi}(t) \\ \hat{z}(t) \end{pmatrix} = \begin{pmatrix} \cosh(\lambda t) & \lambda \sinh(\lambda t) \\ \lambda^{-1}\sinh(\lambda t) & \cosh(\lambda t) \end{pmatrix} \begin{pmatrix} \hat{\varphi} \\ \hat{z} \end{pmatrix}. \quad \text{(E1)}$$

For the OTOC given in the main text one therefore finds

$$C(t) = -\langle [\hat{z}(t), \hat{z}]^2 \rangle \approx \left(\frac{\hbar_{\mathrm{eff}}}{\lambda}\sinh(\lambda t)\right)^2. \quad \text{(E2)}$$

In the case of the three-site BH model one obtains (with the conventions of the last section)

$$|\langle 1,0|\hat{z}_1(t)|0\rangle|^2 = \frac{4\hbar_{\mathrm{eff}}}{3\lambda}\frac{|\cosh(\lambda t + i\phi)|^2}{\sin 2\phi}, \quad \text{(E3)}$$

where $\phi = \tan^{-1}(\omega/\lambda)$ with $\omega = \sqrt{9 - 12\alpha_0}$ and $\lambda = \sqrt{12\alpha_1 - 9}$ for the pre- and post-quench system. Care has to be taken when comparing this result to the quantum-mechanical matrix elements, as the eigenstates of the system are degenerate due to the symmetry of the system. The state $|1,0\rangle$ introduced here does not respect the rotational symmetry of the three-site BH model but is a symmetric superposition of two states with well-defined rotational symmetry $\hat{R}|\Psi_\pm\rangle = e^{\pm 2\pi i/3}|\Psi_\pm\rangle$, where the operator $\hat{R}$ shifts the sites $i \mapsto i+1$. Therefore, a factor 1/2 has been introduced to Eq. (E3) for comparison in Fig. 3 of the main text, where the state $|1,0\rangle$ corresponds to an eigenstate of $\hat{R}$.


[1] Q. Hummel, B. Geiger, J. D. Urbina, and K. Richter, Reversible Quantum Information Spreading in Many-Body Systems near Criticality, Phys. Rev. Lett. **123**, 160401 (2019).

[2] H. Jasiulewicz and W. Kordecki, Convolutions of Erlang and of Pascal Distributions with Applications to Reliability, Demonstr. Math. **36**, 231 (2003).

[3] G. S. James and A. J. Mayne, Cumulants of Functions of Random Variables, Sankhyā A (1961-2002) **24**, 47 (1962).

[4] A. L. Fetter and J. D. Walecka, *Quantum Theory of many-particle Systems*, International Series in pure and appled Physics (McGraw-Hill Book Company, 1971).
